# Supplementary material for: Fast and Universal Kohn Sham Density Functional Theory Algorithm for Warm Dense Matter to Hot Dense Plasma
Source: arXiv:2004.02818 ancillary file (2020-07-24)
Supplement: Supplementary file 1 [file uDFT_supplemental.pdf]

# A Fast and Universal Kohn Sham Density Functional Theory Algorithm for Warm Dense Matter to Hot Dense Plasma: Supplementary Materials

A. J. White[1] and L. A. Collins[1]

[1] *Theoretical Division, Los Alamos National Laboratory, Los Alamos, 87545 NM*

(Dated: June 25, 2020)

## THE MIXED STOCHASTIC-DETERMINISTIC IDENTITY OPERATOR FOR NON-INTERACTING (KOHN-SHAM) WAVEFUNCTIONS

We assume non-interacting systems, such as at the Kohn-Sham, Hartree, or Hartree-Fock level. $\psi$ is an effective or actual single-particle wavefunction, *i.e.* eigenstates of an effective or actual single-particle time-independent Hamiltonian, $\hat{H}$, and the Identity operator can be expressed as:

$$\hat{I} = \sum_{i}^{N_\psi \to \infty} |\psi_i\rangle\langle\psi_i| \tag{1}$$

The stochastic orbitals are defined as:

$$\langle\vec{r}|\chi_b\rangle = e^{i2\pi\theta_b(\vec{r})}/\sqrt{N_\chi d\vec{r}^{\,3}} \tag{2}$$

where $\theta_b(\vec{r})$ is a random number between 0 and 1 specified for each grid point of $\vec{r}$, where $d\vec{r}^{\,3}$ is the volume of a grid element. These random vectors can expressed in terms of $\psi$:

$$|\chi_b\rangle = \sum_{i}^{N_\psi \to \infty} |\psi_i\rangle\langle\psi_i|\chi_b\rangle, \text{ and} \tag{3}$$

$$\langle\psi_i|\chi_b\rangle \equiv c_{i,b} = 1/\sqrt{N_\chi d\vec{r}^{\,3}} \times \int dr' e^{i2\pi\theta_b(\vec{r}')}\psi_i^*(\vec{r}') \tag{4}$$

The equivalence of the fully stochastic Identity operator and the eigenstate based operator is shown by:

$$\begin{aligned}\hat{I} &= \sum_{b}^{N_\chi \to \infty} |\chi_b\rangle\langle\chi_b| = \sum_{b}^{N_\chi \to \infty}\sum_{i,j}^{N_\psi \to \infty} |\psi_i\rangle\langle\psi_i|\chi_b\rangle\langle\chi_b|\psi_j\rangle\langle\psi_j| \\ &= \sum_{i,j}^{N_\psi \to \infty} |\psi_i\rangle\langle\psi_j| \int d\vec{r}' \int d\vec{r}\,\langle\psi_i|\vec{r}'\rangle \frac{1}{N_\chi d\vec{r}^{\,3}} \sum_{b}^{N_\chi \to \infty} e^{i2\pi[\theta_b(\vec{r}')-\theta_b(\vec{r})]}\langle\vec{r}|\psi_j\rangle\end{aligned} \tag{5}$$

Owing to the independence of the random numbers, $\theta$, in the limit of infinite $N_\chi$ we have:

$$\frac{1}{N_\chi d\vec{r}^{\,3}} \sum_{b}^{N_\chi \to \infty} e^{i2\pi[\theta_b(\vec{r}')-\theta_b(\vec{r})]} = \delta(r, r') \tag{6}$$

and thus:

$$\hat{I} = \sum_{b}^{N_\chi \to \infty} |\chi_b\rangle\langle\chi_b| = \sum_{i,j}^{N_\psi \to \infty} |\psi_i\rangle\langle\psi_j|\langle\psi_i|\psi_j\rangle = \sum_{i}^{N_\psi \to \infty} |\psi_i\rangle\langle\psi_i| = \hat{I} \tag{7}$$

From this definition of the identity operator one can build the stochastic DFT approach, and demonstrate its equivalence to the usual Kohn Sham DFT approach in the limit of large stochastic vectors.

Using Eq. 7 and the orthogonormality of the eigenvectors, one can build a mixed identity operator by manipulating the identities:

$$\hat{I} = \sum_{i}^{N_\psi} |\psi_i\rangle\langle\psi_i| + \hat{I} - \sum_{j}^{N_\psi} |\psi_j\rangle\langle\psi_j| \tag{8}$$

$$\hat{I} - \sum_{j}^{N_\psi} |\psi_j\rangle\langle\psi_j| = (\hat{I} - \sum_{j}^{N_\psi} |\psi_j\rangle\langle\psi_j|)(\sum_{b}^{N_\chi\to\infty} |\chi_b\rangle\langle\chi_b|) \equiv \sum_{b}^{N_\chi\to\infty} |\tilde{\chi}_b\rangle\langle\chi_b| \tag{9}$$

$$\sum_{b}^{N_\chi\to\infty} |\tilde{\chi}_b\rangle\langle\chi_b| = \sum_{b}^{N_\chi\to\infty} |\tilde{\chi}_b\rangle\langle\tilde{\chi}_b| + \sum_{b}^{N_\chi\to\infty} \sum_{j}^{N_\psi} |\tilde{\chi}_b\rangle\langle\chi_b|\psi_j\rangle\langle\psi_j|$$

$$\sum_{b}^{N_\chi\to\infty} \sum_{j}^{N_\psi} |\tilde{\chi}_b\rangle\langle\chi_b|\psi_j\rangle\langle\psi_j| = \sum_{b}^{N_\chi\to\infty} \sum_{j}^{N_\psi} |\chi_b\rangle\langle\chi_b|\psi_j\rangle\langle\psi_j| - \sum_{b}^{N_\chi\to\infty} \sum_{j,i}^{N_\psi} |\psi_i\rangle\langle\psi_i|\chi_b\rangle\langle\chi_b|\psi_j\rangle\langle\psi_j| = 0 \tag{10}$$

Combining Eq. 8, 9 and 10 yields the mixed the mixed identity operator

$$\hat{I} = \sum_{i}^{N_\psi} |\psi_i\rangle\langle\psi_i| + \sum_{b}^{N_\chi\to\infty} |\tilde{\chi}_b\rangle\langle\tilde{\chi}_b| \tag{11}$$

## ADDITIONAL VELOCITY AUTOCORRELATION FUNCTIONS (VACF) CALCULATIONS AND DETAILS.

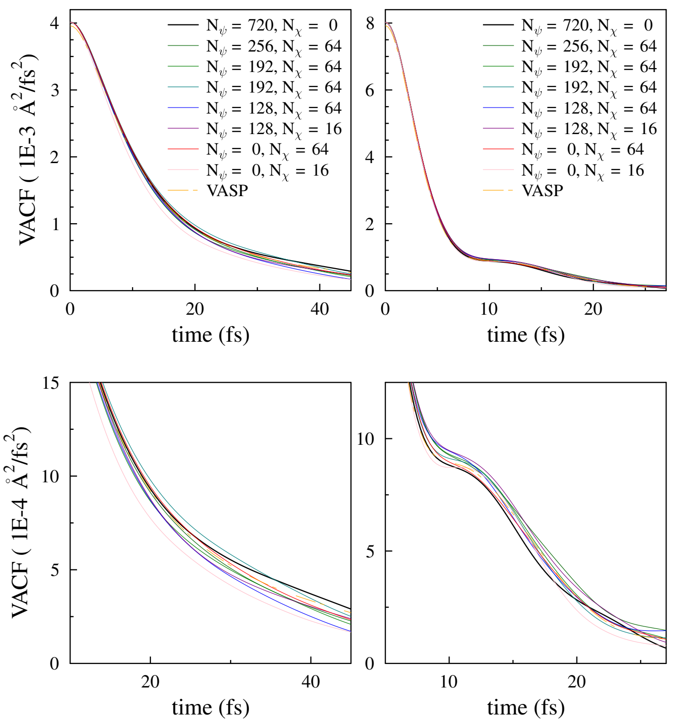


FIG. 1: (Color online)
VACFs for 10 g/cc 10eV (right) and 3.51 g/cc 5eV carbon (left). Lower panels show magnified view of the tail regions where deviations begin to appear.

We have performed additional molecular dynamics simulations, varying only $N_\psi$ and $N_\chi$. The resulting VACFs, Diffusion Coefficients (D), and Free energies (A) are shown in supplemental Figures 1 and Tables I and II. With the

exception of the $N_\psi = 0$ and $N_\chi = 16$ calculation, no significant differences exist based on our 1.8 ps MD trajectories. Our VACFs and D are calculated from the ion velocities ($v_a$) as

$$\vec{V}(t) = 1/N_a \sum_a \vec{v}_a(t) \tag{12}$$

$$VACF(t) = dt/(3N_{t_0}) \sum_{t_0} \vec{V}(t_0) \cdot \vec{V}(t_0 + t) \tag{13}$$

$$D = dt \sum_t VACF(t) \tag{14}$$

where the sum over $t_0$ includes every timestep except for an initial exclusion of 320 and 324 pre-equilibration time steps for the 10eV and 5eV cases respectively. Thus the average VACF's includes $N_{t_0}$ overlapping individual VACFs. This overlap must be accounted for when estimating the error in the VACF / Diffusion coefficient. For calculating the standard error from the standard deviation, one needs to divide by square root of the number of independent samples. Taking $t_0$ at every time point leads to a smoother VACF by averaging over some fast noise, but samples are not fully independent. Thus one needs estimate the number of independent samples by estimating a decorrelation time, $t_D$.

$$St.Error = St.Dev/\sqrt{\frac{N_{t_0} dt}{t_D}} \tag{15}$$

A typical option for $t_D$ is twice the half-life of the average VACF [1], $t_D = 2\tau$, a more conservative option would be the full length of the VACF window, $t_D \sim 10\tau$. In Figure 3 of the main text we have used the first option, in Tables 1 and 2, we have included both. We have repeated the $N_\psi = 192$ $N_\chi = 64$ calculation. We have also compared to a calculation using VASP, and see little difference based on the PAW (VASP) vs HGH (all other) pseudopotentials.

| $N_\psi : N_\chi$ | $A(eV)$ | St.Dev $A(eV)$ | $D(cm^2/s)$ | St.Dev $D(cm^2/s)$ | St.Error $D$ $2\tau$ | St.Error $D$ $10\tau$ |
|---|---|---|---|---|---|---|
| 0 : 16 | -1.4756E+02 | 2.2912E+00 | 4.07E-03 | 1.16E-03 | 7.80E-05 | 1.74E-04 |
| 0 : 64 | -1.4957E+02 | 1.3775E+00 | 4.16E-03 | 1.19E-03 | 7.99E-05 | 1.79E-04 |
| 128 : 16 | -1.5010E+00 | 9.2596E-01 | 4.22E-03 | 1.22E-03 | 8.21E-05 | 1.84E-04 |
| 128 : 64 | -1.5005E+02 | 9.2080E-01 | 4.23E-03 | 1.22E-03 | 8.21E-05 | 1.84E-04 |
| 192 : 64 | -1.5013E+02 | 8.9671E-01 | 4.26E-03 | 1.22E-03 | 8.23E-05 | 1.84E-04 |
| 192 : 64 | -1.5016E+02 | 8.8131E-01 | 4.22E-03 | 1.27E-03 | 8.52E-05 | 1.90E-04 |
| 256 : 64 | -1.5019E+02 | 9.1441E-01 | 4.25E-03 | 1.20E-03 | 8.07E-05 | 1.81E-04 |
| 720 : 0 | -1.5009E+02 | 9.2278E-01 | 4.10E-03 | 1.24E-03 | 8.31E-05 | 1.86E-04 |

TABLE I: 10g/cc 10 ev, $\tau = 4.25$ fs, dt=0.25 fs, total time = 1.8 ps, $N_{t_0} = 6720$.

| $N_\psi : N_\chi$ | $A(eV)$ | St.Dev $A(eV)$ | $D(cm^2/s)$ | St.Dev $D(cm^2/s)$ | St.Error $D$ $2\tau$ | St.Error $D$ $10\tau$ |
|---|---|---|---|---|---|---|
| 0 : 16 | -1.5793E+02 | 1.1581E+00 | 5.49E-03 | 1.42E-03 | 1.87E-04 | 4.19E-04 |
| 0 : 64 | -1.5880E+02 | 6.4184E-01 | 6.14E-03 | 1.43E-03 | 1.88E-04 | 4.20E-04 |
| 128 : 16 | -1.5918E+02 | 3.5038E-01 | 6.06E-03 | 1.24E-03 | 1.63E-04 | 3.65E-04 |
| 128 : 64 | -1.5916E+02 | 3.5446E-01 | 5.79E-03 | 1.40E-03 | 1.84E-04 | 4.12E-04 |
| 192 : 64 | -1.5923E+02 | 3.2554E-01 | 5.88E-03 | 1.26E-03 | 1.65E-04 | 3.70E-04 |
| 192 : 64 | -1.5925E+02 | 3.1371E-01 | 6.27E-03 | 1.17E-03 | 1.54E-04 | 3.43E-04 |
| 256 : 64 | -1.5927E+02 | 3.2888E-01 | 6.09E-03 | 1.33E-03 | 1.76E-04 | 3.93E-04 |
| 720 : 0 | -1.5923E+02 | 3.1831E-01 | 6.23E-03 | 1.16E-03 | 1.52E-04 | 3.40E-04 |

TABLE II: 3.51g/cc 5 eV. $\tau = 13.5$ fs, dt=0.5 fs, total time = 1.8 ps, $N_{t_0} = 3114$.

## EARLY TIME (NONEQUILLIBRIUM) MOLECULAR DYNAMICS COMPARISONS FROM VACF CALCULATIONS

Since all our KS-DFT MD calculations were originated from the same initial positions, we can flow the time dependent free energy to determine how long before the stochastic force errors lead to a change in the trajectory. This can give us a simpler view for comparison of the accuracies without convoluting molecular dynamics sampling error (based on the overall length of the trajectory). We plot the results in Figure 2 and 3. This portion of the trajectory is discarded from the VACF calculations in Figure 3 of the main text. It is clear that the more accurate (higher $N_\chi$ and $N_\psi$) mDFT calculation follows the dDFT calculation than the less accurate mDFT. The sDFT calculations show more significant fluctuations. The $N_\chi = 16$ sDFT calculation shows a significant difference in the average free energy as well, indicating large nonlinear bias. This supports our conclusion that while the lower accuracy calculations may agreed better with dDFT simulations in Figure 3 of the main text, this is due to molecular dynamics convergence.

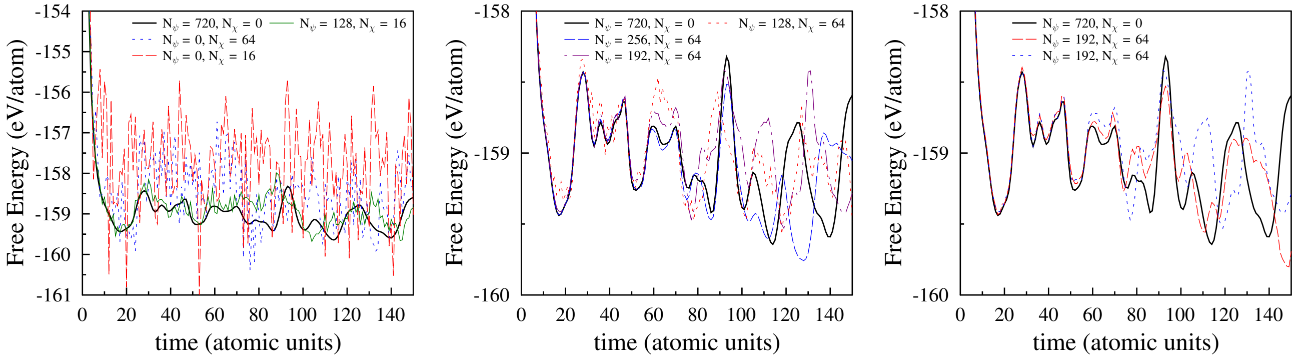


FIG. 2: (Color online)
Time dependent Free energy showing relaxation from initial positions. 3.51 g/cc 5eV carbon.

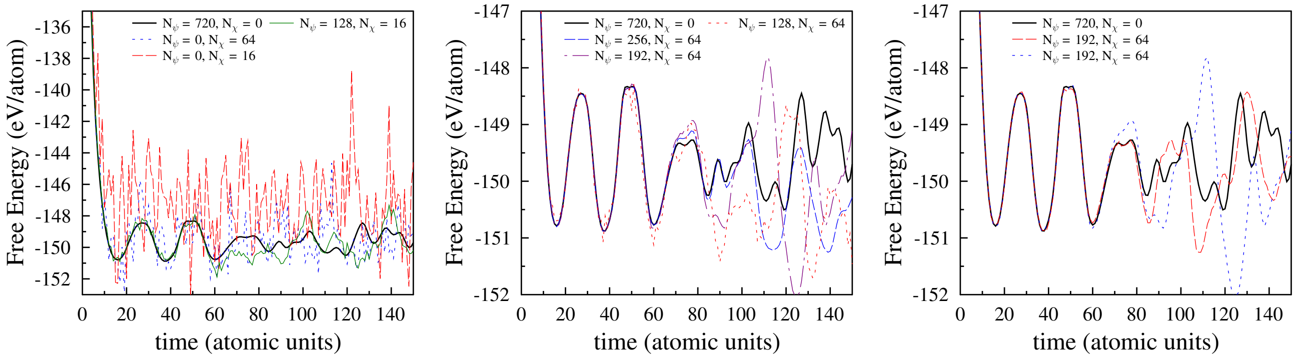


FIG. 3: (Color online)
Time dependent Free energy showing relaxation from initial positions. 10 g/cc 10eV carbon.

## SIMULATION DETAILS

| Figure: | 1 | 2 | 3 Letter & 1-3 SM (Sim 1) | 3 Letter & 1-3 SM (Sim 2) |
|---|---|---|---|---|
| Material: | Carbon | Carbon | Carbon | Carbon |
| Structure: | Diamond | Disordered | Disordered | Disordered |
| Density: | 3.51 g/cc | 3.51 g/cc | 3.51 g/cc | 10 g/cc |
| Temperature: | 10 eV | 3-50 eV | 5 eV | 10 eV |
| KS-DFT Exchange Correlation: | PBE GGA [2] | PBE GGA [2] | PBE GGA [2] | PBE GGA [2] |
| OF-DFT Kinetic Energy: | TFP [4] | N/A | N/A | N/A |
| OF-DFT Exchange Correlation: | PZCA [5] | N/A | N/A | N/A |
| Number of atoms: | 64 | 64 | 64 | 64 |
| K-points: | 1 (Γ) | 1 (Γ) | 1 (Γ) | 1 (Γ) |
| Planewaves: | $96^3$ | $64^3$ | $64^3$ | $48^3$ |
| Broadening ($\gamma$): | 2 eV | N/A | N/A | N/A |
| Pseudopotential : | HGH 4e- Carbon [3] | HGH 4e- Carbon [3] | HGH 4e- Carbon [3] | HGH 4e- Carbon [3] |
| VASP Pseudopotential : | N/A | N/A | see caption | see caption |
| dDFT $N_\psi$: | 1280 | Table 1, Letter | 720 | 720 |
| sDFT: $N_\chi$: | 128 | 128 | 16 & 64 | 16 & 64 |
| mDFT: $N_\psi/N_\chi$ | 128/64 | Table 1, Letter | Fig. 3 key, Letter | Fig. 3 key, Letter |

TABLE III: Simulation details: VASP Pseudopotential PAW 4e- Carbon (hard, EMAX 700) $\text{PAW}_{PBE}$ $C_h$ 06Feb2004 for 4 electrons s2p2


[1] E. R. Meyer, J. D. Kress, L. A. Collins, and C. Ticknor, Phys. Rev. E. **90**, 043101 (2014).
[2] J. P. Perdew, K. Burke, and M. Ernzerhof, Phys. Rev. Lett. **77**, 3865 (1996).
[3] C. Hartwigsen, S. Goedecker, and J. Hutter, Phys. Rev. B **58**, 3641 (1998).
[4] F. Perrot, Physical Review A **20**, 586 (1979).
[5] J. P. Perdew and A. Zunger, Phys. Rev. B **23**, 5048 (1981).
